# Supplementary material for: Phase-Coherent Spin and Lattice Modulations in a Y-type Hexaferrite
Source: arXiv:2610.17292 source file (2026-10-12)
Supplement: Supplementary file 1 [file SM_latest.tex]

%\documentclass[aps,prl,onecolumn,superscriptaddress,floatfix,nofootinbib]{revtex4-2}

%\usepackage{graphicx}
%\usepackage{amsmath}
%\usepackage{amssymb}
%\usepackage{bm}
%\usepackage{float}
%% Float placement for the one-column supplement: figures at page tops, at most two
%% per page, so that each is legible and the text is not fragmented.
%\renewcommand{\topfraction}{0.88}
%\renewcommand{\bottomfraction}{0.70}
%\renewcommand{\textfraction}{0.10}
%\renewcommand{\floatpagefraction}{0.70}
%\setcounter{topnumber}{2}
%\setcounter{bottomnumber}{1}
%\setcounter{totalnumber}{2}
%
%\newcommand{\BSMFO}{Ba$_{0.4}$Sr$_{1.6}$Mg$_2$Fe$_{12}$O$_{22}$}
%\newcommand{\kZ}{k_{0}}
%\newcommand{\kT}{k_{2}}
%\newcommand{\kTh}{k_{3}}
%\newcommand{\rlu}{\text{r.l.u.}}
%\newcommand{\Phat}{\hat{\bm{P}}}
%\newcommand{\Qhat}{\hat{\bm{Q}}}
%\newcommand{\Mperp}{\bm{M}_{\perp}}
%\newcommand{\MH}{M_{\parallel H}}
%
%\renewcommand{\thefigure}{S\arabic{figure}}
%\renewcommand{\thetable}{S\Roman{table}}
%\renewcommand{\theequation}{S\arabic{equation}}
%
%\begin{document}

\title{Supplemental Material:\\
Phase-Coherent Spin and Lattice Modulations in a Y-type Hexaferrite}

\author{O. Stepančić}
\affiliation{Division of Synchrotron Radiation Research, Department of Physics,
Lund University, SE-22100 Lund, Sweden}

\author{A. Stellhorn}
\affiliation{European Spallation Source ERIC, Partikelgatan 2, 224 84 Lund, Sweden}

\author{E. Campillo}
\affiliation{Division of Synchrotron Radiation Research, Department of Physics,
Lund University, SE-22100 Lund, Sweden}

\author{K. Zhai}
\affiliation{Center for High Pressure Science, State Key Laboratory of Metastable Materials
Science and Technology, Yanshan University, Qinhuangdao, China}

\author{N. Ekström}
\affiliation{European Spallation Source ERIC, Partikelgatan 2, 224 84 Lund, Sweden}

\author{A. Corani}
\affiliation{European Spallation Source ERIC, Partikelgatan 2, 224 84 Lund, Sweden}

\author{D. Alba Venero}
\affiliation{ISIS neutron and muon source, STFC, Rutherford Appleton Laboratory, Didcot OX11 0QX, United Kingdom}

\author{R. Cubitt}
\affiliation{Institut Laue--Langevin, CS 20156, 38042 Grenoble Cedex 9, France}

\author{E. Blackburn}
\email{elizabeth.blackburn@fysik.lu.se}
\affiliation{Division of Synchrotron Radiation Research, Department of Physics,
Lund University, SE-22100 Lund, Sweden}

\author{L. Shen}
\email{lingjia.shen@fysik.lu.se}
\affiliation{Division of Synchrotron Radiation Research, Department of Physics,
Lund University, SE-22100 Lund, Sweden}

% \date{\today}

\maketitle

\section{Data Reduction and Profile Analysis}
\label{sec:reduction}

Longitudinal profiles were extracted in two stages. First, the reconstructed reciprocal-space map was divided into rows of constant $L$, and the transverse intensity distribution in each row was fitted with a Gaussian function on a constant background,
\begin{equation}
I(H)=B+\frac{A}{\sigma_H\sqrt{2\pi}}\exp\!\left[-\frac{(H-H_0)^2}{2\sigma_H^2}\right].
\end{equation}
The peak center and width were constrained to $|H_0|\leq3\times10^{-3}$~\rlu\ and $\sigma_H\leq2\times10^{-3}$~\rlu, with these bounds chosen according to the reciprocal-space binning. The fitted area $A$ gives the intensity assigned to that row, so the resulting longitudinal profile $A(L)$ is constructed from intensities integrated across the transverse direction rather than from peak heights within a single narrow column of pixels. Second, $A(L)$ was fitted with a sum of Gaussians,
\begin{equation}
A(L)=C+\sum_{\alpha}\sum_{j=1}^{n_{\alpha}}
\frac{a_{\alpha j}}{\sigma_{\alpha j}\sqrt{2\pi}}
\exp\!\left[-\frac{(L-L_{0,\alpha})^{2}}{2\sigma_{\alpha j}^{2}}\right],
\qquad
\sigma_{\alpha j}=\frac{w_{\alpha j}}{2\sqrt{2\ln2}},
\end{equation}
where $\alpha\in\{\kZ,\kT,\kTh\}$ labels the scattering component and $j$ labels the Gaussian contributions assigned to it. The $\kZ$ and $\kT$ components were each represented by a narrow Gaussian and a diffuse Gaussian sharing a common center, whereas $\kTh$ was represented by a single Gaussian. The center of $\kZ$ was refined, while those of $\kT$ and $\kTh$ were fixed at $L=1.5$ and $L=1.65$, respectively. Allowing the $\kT$ and $\kTh$ centers to vary freely produced values consistent with these positions and did not change the fitted intensities or asymmetries within uncertainty. Here, $a_{\alpha j}$ is the integrated area and $w_{\alpha j}$ is the full width at half maximum. The two incident-neutron polarization channels were fitted jointly: the centers and widths of each Gaussian were shared between channels, because both channels probe the same underlying structure, while the integrated areas $a_{\alpha j}^{+}$ and $a_{\alpha j}^{-}$ were allowed to differ. For a component containing more than one Gaussian, its total integrated intensity, which is used in the main text ($I^{\pm}$), was obtained by summing the corresponding areas, $a_{\alpha}^{\pm}=\sum_j a_{\alpha j}^{\pm}$. The polarization asymmetry was then calculated as $r_{\alpha}=(a_{\alpha}^{+}-a_{\alpha}^{-})/(a_{\alpha}^{+}+a_{\alpha}^{-})$. Because it is defined from integrated areas, $r_{\alpha}$ is independent of the fitted longitudinal widths by construction and can therefore be compared directly across fields and temperatures for which the linewidths vary.



\subsection*{Polarization and instrumental controls}

Because the central conclusion rests on a large polarization asymmetry, the controls deserve to be stated explicitly. Two points bear on whether the asymmetry could be instrumental.

First, the vanishing asymmetry at $\kT$ should not be interpreted as evidence that the $\kT$ order is nonchiral. In $R\bar{3}m$, allowed reciprocal-lattice vectors along $\bm c^{*}$ have $L=3n$. Because $\kT=(0,\,0,\,1.5)$ \cite{Zhai2017},
\begin{equation}
2\kT=(0,\,0,\,3)=\bm G,\qquad \kT\equiv-\kT\pmod{\bm G}.
\end{equation}
The $\kT$ satellite therefore lies at the zone boundary: the satellite generated as $0+\kT$ coincides with that generated as $(0,\,0,\,3)-\kT$. Unlike the $\kTh$ modulation, whose conjugate satellites are resolved at $L=1.35$ and $L=1.65$, $\kT$ has no spatially separated pair at which the even and odd parts of the polarization asymmetry can be compared. Consequently, the conjugate-satellite parity test used in Fig.~4 of the main text cannot distinguish nuclear-magnetic interference from magnetic chirality at $\kT$. The observation $r(\kT)\simeq0$ establishes only that no net polarization-dependent contribution is resolved in the present geometry; it does not by itself constrain the chirality of the $\kT$ state. Nevertheless, $\kT$ remains a useful instrumental null: its asymmetry is consistent with zero throughout the same measurements and under the same analysis procedure for which $\kTh$ exhibits a large positive asymmetry. This comparison shows that the $\kTh$ asymmetry is not a generic offset introduced by the polarization setup, normalization, or profile fitting.

Second, finite incident polarization and flipper efficiency reduce the measured asymmetry by an effective multiplicative factor, $r_{\mathrm{obs}}=\mathcal{P}_{\mathrm{eff}}r$, with $\mathcal{P}_{\mathrm{eff}}\leq1$. The physical asymmetry is therefore at least as large as the observed value, making all bounds obtained directly from $r_{\mathrm{obs}}$ conservative. In particular, $r_{\mathrm{obs}}\leq|\cos\varphi|$ remains valid, so correcting for finite polarization could only tighten the phase bound, while $f_{\perp}\leq1-r_{\mathrm{obs}}^{2}$ remains a valid upper limit on the noninterfering magnetic fraction. We therefore apply no polarization correction and quote conservative limits obtained by treating the observed asymmetry as its ideal-instrument value.

\section{Flipper-independent counterparts of the main-text figures}

\begin{figure}[H]
\centering
\includegraphics[width=0.85\textwidth]{figs/FigureS1_RSM_profiles_flipperminus.pdf}
\caption{As Fig.~1 of the main text, for the $I^{-}$ polarization channel. Colour scales are
identical to the corresponding $I^{+}$ panels.}
\label{fig:S1}
\end{figure}

\begin{figure}[H]
\centering
\includegraphics[width=0.45\textwidth]{figs/FigureS2_field_flipperminus.pdf}
\caption{As Fig.~3 of the main text, for the $I^{-}$ polarization channel.}
\label{fig:S2}
\end{figure}


Figures~1 and~3 of the main text show the $I^{+}$ channel only. Figures~\ref{fig:S1}
and~\ref{fig:S2} give the $I^{-}$ counterparts. The reciprocal-space maps use the same
per-field colour scale as the corresponding $I^{+}$ panels, so the two figures may be compared
directly; the $\kTh$ satellite is visibly weaker in $I^{-}$, which is the asymmetry reported
in the main text.

\section{Per-component field and temperature dependences}

\begin{figure}[H]
\centering
\includegraphics[width=0.9\textwidth]{figs/FigureS3_k0_components.pdf}
\caption{Field dependence of the $\kZ$ narrow and diffuse integrated areas and their fitted full widths at half maximum. }
\label{fig:S3}
\end{figure}

\begin{figure}[H]
\centering
\includegraphics[width=0.9\textwidth]{figs/FigureS4_k2_components.pdf}
\caption{Field dependence of the $\kT$ core and diffuse integrated areas.}
\label{fig:S4}
\end{figure}

The three components of the $(0,\,0,\,L)$ scattering -- $\kZ\approx(0,\,0,\,1.03)$, $\kT=(0,\,0,\,1.5)$, and $\kT=(0,\,0,\,1.65)$-- were separated by joint fits to the complete field or temperature series, as described in the first section. An $L$-independent term accounts for residual rod scattering along $H=0$. The assignments of $\kZ$ and $\kT$ to longitudinal-conical and twofold transverse-conical orders, respectively, follow the magnetic structures established for this family by neutron and resonant x-ray diffraction~\cite{Zhai2017}. In the constrained field-series analysis, the $\kTh$ component was included from $2$~T upward. Introducing this component at lower fields does not significantly improve the fit and yields no resolved polarization dependence. Because broad $\kTh$-like scattering may remain indistinguishable from the diffuse tail of the much stronger $\kT$ component, these results establish the positive identification of a distinct, polarization-dependent $\kTh$ satellite above approximately $2$~T within our detection limit.

Figures~\ref{fig:S3} and~\ref{fig:S4} show the field dependence of the narrow and diffuse $\kZ$ and $\kT$ components and their linewidths, while Fig.~\ref{fig:S6} shows the temperature dependence of the two $\kT$ components. Figures~\ref{fig:S5} and~\ref{fig:S7} show the field and temperature dependence of the $\kTh$ linewidth: it narrows with increasing field, varies little above ${\sim}3$~T, and is essentially temperature independent at $7$~T. The $\kTh$ integrated area at $7$~T decreases by a factor of $4.2$ between $15$ and $275$~K, from $1.63\times10^{-3}$ to $3.89\times10^{-4}$ in Fig.~2(b), main text, while its asymmetry increases from $0.819$ to $0.910$. This is the fourfold decrease quoted in the main text and demonstrates that the strong polarization-dependent interference persists as the total satellite intensity declines. Two further consequences of the decomposition are used in the main text. First, the $\kT$ intensity decreases by several orders of magnitude and becomes indistinguishable from zero by $6$~T, whereas $\kTh$ persists to at least $7$~T. Because the uniform magnetization is already close to its extrapolated ferrimagnetic value at this field (Fig.~\ref{fig:S8}), a well-defined incommensurate modulation coexists with a large uniform magnetization, demonstrating that the high-field state is not a simple uniform ferrimagnet. We avoid describing the measured magnetization as saturated because a finite high-field slope remains; throughout, $M_{\mathrm{sat}}$ denotes the zero-field intercept of a linear fit to the high-field region, i.e., the extrapolated ferrimagnetic moment. Second, the $\kTh$ linewidth narrows with increasing field and then changes little above ${\sim}3$~T (Fig.~\ref{fig:S5}), while remaining essentially temperature independent at $7$~T (Fig.~\ref{fig:S7}). This behaviour differs from that of $\kT$, whose diffuse component persists to high temperature (Fig.~\ref{fig:S6}). 

\begin{figure}[t]
\centering
\includegraphics[width=0.9\textwidth]{figs/FigureS6_k2_components_vsT.pdf}
\caption{Temperature dependence of the $\kT$ core and diffuse integrated areas at $1$~T.}
\label{fig:S6}
\end{figure}


\begin{figure}[H]
\centering
\includegraphics[width=0.45\textwidth]{figs/FigureS5_k3_FWHM.pdf}
\caption{Fitted full width at half maximum of the $\kTh$ satellite against field.}
\label{fig:S5}
\end{figure}

\begin{figure}[H]
\centering
\includegraphics[width=0.45\textwidth]{figs/FigureS7_k3_FWHM_vsT.pdf}
\caption{Fitted full width at half maximum of the $\kTh$ satellite at $7$~T against
temperature.}
\label{fig:S7}
\end{figure}

\section{Bulk magnetization}

\begin{figure}[H]
\centering
\includegraphics[width=0.60\textwidth]{figs/FigureS8_MH_5K.pdf}
\caption{$M$-$H$ loop at $5$~K, with the initial (virgin), descending and ascending branches labelled separately. Green dashed line, the high-field linear fit whose intercept gives $M_{\mathrm{sat}}$. Inset, magnification of the $-0.05$ to $0.4$~T region.}
\label{fig:S8}
\end{figure}

Figure~\ref{fig:S8} shows the $M$-$H$ loop at $5$~K in units of Bohr magnetons per formula unit. The measurement followed the sequence $0\rightarrow+7\rightarrow-7\rightarrow+7$~T and therefore includes a virgin branch that is not retraced in the subsequent loop. Two quantities extracted from this measurement are used in the main text. First, the magnetization remains field-dependent at $7$~T and therefore does not reach strict saturation within the measured range. Accordingly, $M_{\mathrm{sat}}$ is estimated from the zero-field intercept of a linear fit to the high-field region, giving $M_{\mathrm{sat}}=9.15\pm0.01\,\mu_{\mathrm B}$/f.u.. Second, along the virgin branch, $M(H\rightarrow0)=-0.04\,\mu_{\mathrm B}$/f.u., while the magnetization reaches $87\%$ of the extrapolated $M_{\mathrm{sat}}$ by $2$~T, the field range over which the coherent $\kTh$ state becomes clearly identifiable. The quoted $87\%$ is referenced to the extrapolated ferrimagnetic moment, not to a saturation value directly attained in the experiment. The value $M_{\mathrm{sat}}=9.15\,\mu_{\mathrm B}$/f.u. is not anomalously low and does not, by itself, provide evidence for spin canting. For twelve Fe$^{3+}$ ions per formula unit and nonmagnetic Mg, the collinear ferrimagnetic arrangement gives a net moment of $2m(\mathrm{Fe}^{3+})$, corresponding to $10\,\mu_{\mathrm B}$/f.u. for the spin-only value $m(\mathrm{Fe}^{3+})=5\,\mu_{\mathrm B}$. The extrapolated moment instead corresponds to $m(\mathrm{Fe}^{3+})=4.575\,\mu_{\mathrm B}$, a modest reduction compatible with ordinary covalency and orbital effects.

\section{Upper limit on the $G= (0,\,0,\,0)$ satellite and the intensity ratio}
\label{sec:limit}

The main text reports that satellites around $\bm G=(0,\,0,\,3)$ are clearly resolved, whereas only a marginal excess is seen around $\bm G=(0,\,0,\,0)$, and quotes the polarization-summed integrated-intensity ratio $I(1.65)/I(1.35)>18$, with a conservative bound of $12$. Both limits are derived below. Importantly, the $\bm G=(0,\,0,\,0)$ satellite is bounded rather than shown to vanish; the analysis therefore yields a one-sided upper limit at a specified confidence level. We use the $15$~K profile from the $7$~T temperature scan, which spans $L=0.56$--$1.84$ and contains both satellite positions within the same measurement. A $23$-point baseline over $0.56<L<1.30$ constrains the background independently of either satellite. The reference model consists of the $\kTh$ satellite and a constant background, with no $\kT$ contribution. To this model we add a candidate satellite at $L=1.35$, with its center fixed by the conjugate position and its width tied to that refined for $\kTh$ at $L=1.65$. Tying the widths prevents a fit in a peak-free region from converging on a narrow statistical fluctuation and returning an artificially small integrated area. The candidate area ($a_{35}$) is the only additional parameter; at each trial value, the $\kTh$ area, center, and width and the constant background are reoptimized, so the resulting limit accounts for their covariance with $a_{35}$. The reference fit gives $\chi^{2}/\mathrm{dof}=1.02$, with the $\kTh$ center at $L=1.649$~\rlu, a FWHM of $0.1723$~\rlu, and an integrated area of $1.55\times10^{-3}$. Allowing the candidate area to take either sign, the fit returns $a_{35}=5.0(2.1)\times10^{-5}$, a marginal $2.4\sigma$ excess at the conjugate position, with $\chi^{2}/\mathrm{dof}=0.88$; the other temperatures of the same scan give excesses between $-0.6\sigma$ and $+2.8\sigma$, and the width refined at $L=1.35$, $0.19(4)$~\rlu, matches that at $L=1.65$. A satellite at the $\bm G=(0,\,0,\,0)$ position is therefore neither established nor excluded, and we quote one-sided upper limits measured from the best fit,
\begin{equation}
a_{35}<8.4\times10^{-5}\quad(95\%\ \mathrm{CL}),\qquad
a_{35}<1.1\times10^{-4}\quad(3\sigma),
\end{equation}
corresponding to
\begin{equation}
\frac{I(1.65)}{I(1.35)}>18\quad(95\%\ \mathrm{CL}),\qquad
\frac{I(1.65)}{I(1.35)}>14\quad(3\sigma),
\end{equation}
and a central value $I(1.65)/I(1.35)\simeq31^{+21}_{-9}$. Inflating all uncertainties by the factor of approximately two indicated by the intensity dependence of the profile-fit $\chi^{2}$ weakens these limits to $>13$ ($95\%$) and $>9$ ($3\sigma$); we quote $13$ in the main text as the conservative $95\%$-confidence lower bound.

\subsection*{Independent confirmation from ZOOM}
\begin{figure}[H]
\centering
\includegraphics[width=0.55\textwidth]{figs/FigureS9_7T_conjugate_limit.pdf}
\caption{Independent $7$~T/5~K test at ZOOM. Blue circles, $I^{+}$; red squares, $I^{-}$; solid curves, the joint fit with the $\kTh$ center, FWHM and constant background shared between channels and only the integrated areas free; dashed purple line, the shared constant. The green dashed curve shows the $95\%$-confidence upper limit on a satellite at the conjugate position $L=1.35$, with its center fixed and its width tied to that refined at $L=1.65$.}
\label{fig:S9}
\end{figure}


The same bound can be constructed from an independent dataset at 5~K and 7~T collected from the ZOOM instrument at the ISIS Neutron and Muon Facility under the same geometry. Figure~\ref{fig:S9} shows this profile for both polarization channels. The $\kTh$ satellite is centered at $L=1.65$. The two channels are fitted jointly with the $\kTh$ center, the FWHM and the constant background shared between them and only the two integrated areas free, exactly as in the joint two-channel analysis described above.
% ; the fit gives a FWHM of $0.143\pm0.013$~\rlu\ and an asymmetry $r=+0.50\pm0.08$. 
The positive sign of $r$ in an independent reduction is itself a useful control on the interference interpretation, although the value is not identical to that obtained from the D33 measurements ($r=0.75\pm0.06$ at the same field). 

The conjugate position $L=1.35$ lies within the measured range and is subtended by $24$ baseline points below $L=1.30$ that fix the background independently of either satellite. Following the construction above, a candidate Gaussian is placed at $L=1.35$ with its center fixed and its width tied to that refined at $L=1.65$, and its area $a_{35}$ is profiled with the $\kTh$ areas, the shared width and the constant reoptimized at every trial value. The fit returns $a_{35}=0.6(1.0)\times10^{-3}$, consistent with zero, and one-sided limits measured from the best fit give
\begin{equation}
a_{35}<2.2\times10^{-3}\quad(95\%~\mathrm{confidence\ level}),\qquad a_{35}<3.5\times10^{-3}\quad(3\sigma),
\end{equation}
which, against the polarization-summed area $3.14\times10^{-2}$ at $L=1.65$, corresponds to
\begin{equation}
\frac{I(1.65)}{I(1.35)}>14\quad(95\%~\mathrm{confidence\ level}),\qquad \frac{I(1.65)}{I(1.35)}>9\quad(3\sigma).
\end{equation}
These limits are slightly weaker than those derived from D33. They are of the same sense and of the same order, and the ZOOM data show no excess at the conjugate position, so they confirm the zone contrast independently.

\subsection*{From polarization-summed to nuclear intensities}

The bound above applies to the polarization-summed intensity, whereas the rigid-translation prediction concerns the nuclear structure factor. The two can be related through the measured asymmetry, which provides a lower bound on the nuclear fraction of the $L=1.65$ satellite. Summing the two polarization channels eliminates both polarization-dependent terms and gives $I^{+}+I^{-}=2(|N|^{2}+|\Mperp|^{2})$. The upper limit at $L=1.35$ therefore applies to a positive sum of nuclear and magnetic intensities and is, \emph{a fortiori}, an upper limit on the nuclear intensity at that position. At $L=1.65$, Eq.~(2), together with $|M_H|\leq|\Mperp|$ and $|\cos\varphi|\leq1$, gives
\begin{equation}
|r|\leq\frac{2|N||\Mperp|}{|N|^{2}+|\Mperp|^{2}}=\frac{2t}{1+t^{2}},\qquad t\equiv\frac{|\Mperp|}{|N|}.
\end{equation}
The largest ratio compatible with the observed asymmetry is $t_{\max}=[1+\sqrt{1-r^{2}}]/|r|$, yielding the conservative lower bound
\begin{equation}
f_N\equiv\frac{|N|^{2}}{|N|^{2}+|\Mperp|^{2}}\geq\frac{1}{1+t_{\max}^{2}}=\frac{1-\sqrt{1-r^{2}}}{2}.
\end{equation}
This gives $f_N\geq0.17$ for $r=0.75$, $f_N\geq0.21$ for $r=0.819$, and $f_N\geq0.32$ for $r=0.9337$. In particular, the $15$~K asymmetry $r=0.819$, measured for the same profile used to determine the zone contrast, requires at least $21\%$ of the polarization-summed satellite intensity at $L=1.65$ to be nuclear. Combining this result with the nominal 95\%-confidence bound $I(1.65)/I(1.35)>18$ gives
\begin{equation}
\frac{|N(1.65)|^{2}}{|N(1.35)|^{2}}>3.9.
\end{equation}
This nuclear-to-nuclear contrast assumes only the minimum nuclear contribution required by the asymmetry and conservatively treats the entire upper limit at $L=1.35$ as nuclear. Using the uncertainty-inflated intensity ratio of $12$ instead gives a conservative nuclear contrast greater than $2.5$. Destructive nuclear--magnetic interference cannot conceal the $L=1.35$ satellite in this analysis because the limit is obtained from $I^{+}+I^{-}$, in which the interference term cancels identically.


The significance of this bound lies primarily in the direction of the
zone contrast. For a rigid displacement of the crystallographic basis,
$F_N(\bm G+\bm q)\propto iQ\,u_cF_{\mathrm{nuc}}(\bm G)$. Direct
evaluation using the $4$~K refinement of
Ref.~\onlinecite{Zhai2017} gives
$F_{\mathrm{nuc}}(0)=793.8$~fm and
$F_{\mathrm{nuc}}(003)\simeq-66$~fm. The latter value is also obtained
by summing the $C^E_3$ coefficients in Table~\ref{tab:pair} and restoring
the omitted factor of three from $R$ centering. Including the $Q^2$
prefactor therefore gives
\begin{equation}
\frac{I_{\mathrm{rigid}}(1.35)}
{I_{\mathrm{rigid}}(1.65)}
=
\left(\frac{1.35}{1.65}\right)^2
\left|
\frac{F_{\mathrm{nuc}}(0)}
{F_{\mathrm{nuc}}(003)}
\right|^2
\simeq97.
\end{equation}
A rigid displacement would thus make the $\bm G=(0,\,0,\,0)$ satellite
approximately $10^2$ times stronger than the
$\bm G=(0,\,0,\,3)$ satellite. The observed nuclear contrast has the
opposite sense, with
$|N(1.65)|^2/|N(1.35)|^2>3.9$ for the nominal uncertainties and $>2.5$
under the conservative error inflation. The rigid-basis prediction and
the conservative experimental bound therefore differ by a factor
exceeding $2.4\times10^2$. The conclusion that the observed modulation
involves relative displacements within the crystallographic basis does
not depend on assigning the full $L=1.65$ intensity to nuclear
scattering.


\section{Construction of the phase bound}
\label{sec:phase}

Equation~(2) of the main text, evaluated for ideal incident polarization after the conjugate-satellite comparison has identified the asymmetry as predominantly even nuclear-magnetic interference, with no odd chiral contribution resolved, becomes
\begin{equation}
r=\frac{2|N||M_H|\cos\varphi}{|N|^{2}+|M_H|^{2}+|M_{\perp,\not P}|^{2}},
\end{equation}
where $\varphi\equiv\arg(N^{*}M_H)$ and $M_{\perp,\not P}$ denotes magnetic components perpendicular to $\Phat$ that contribute to the total intensity but not to the interference term. Because the amplitude-dependent prefactor cannot exceed unity, every measured asymmetry satisfies $|r|\leq|\cos\varphi|$ and therefore constrains the relative structure-factor phase through $|\varphi|\leq\arccos|r|$. This inequality requires no assumption about the temperature dependence of either amplitude. It is not legitimate, however, to substitute the largest measured asymmetry directly into this relation, because the maximum of a noisy quantity is an upward-biased estimator. Simulations of $23$ measurements with the observed uncertainties and a constant true asymmetry $r=0.80$ give $\max r\geq0.94$ in $13\%$ of trials and $\mathbb{E}[\max r]=0.895$; moreover, the largest observed values occur where the weaker polarization channel is least significant. We therefore use a profile-likelihood construction in which $\cos\varphi$ is the only parameter shared across temperature, while the nuclear and magnetic amplitudes are profiled independently at each of the $n=22$ usable temperatures. This procedure imposes no assumed temperature dependence on either amplitude. Using the nominal $95\%$ threshold $\Delta\chi^{2}=3.84$ gives $|\varphi|\leq24.5^{\circ}$ with the nominal uncertainties and $|\varphi|\leq29.5^{\circ}$ after inflating all uncertainties by a factor of two. Restricting the analysis to the $16$ temperatures for which the weaker polarization channel exceeds three standard deviations relaxes the bound to $|\varphi|\leq32.9^{\circ}$. The main text therefore quotes the conservative rounded limit $|\varphi|\lesssim35^{\circ}$.

\emph{Bootstrap calibration of the likelihood threshold.} Because the amplitudes are profiled independently at each temperature and $\cos\varphi$ is weakly constrained in parts of the nuisance-parameter space, the asymptotic Wilks thresholds need not provide their nominal coverage. We therefore calibrated the profile-likelihood interval by parametric bootstrap. Synthetic $I^{\pm}$ data were generated from the fitted model at a specified value of $\cos\varphi$, refitted using the same procedure as the experimental data, and tested for whether the resulting interval contained the generating value. For $800$ replicas generated at the best-fit value $\cos\varphi=0.97$, all intervals constructed with $\Delta\chi^{2}=3.84$ contained the generating value, while the intervals constructed with $\Delta\chi^{2}=2.71$ gave $99.6\%$ coverage. The threshold required for $95\%$ coverage is therefore smaller than either conventional value, showing that the adopted interval overcovers rather than undercovers. Repeating the calculation for $\cos\varphi=0.92$, $0.95$, $0.98$, and $1.00$ gives median upper limits of $|\varphi|\simeq23^{\circ}$--$25^{\circ}$, compared with $25.8^{\circ}$ obtained from the experimental data using $\Delta\chi^{2}=3.84$. The limit $|\varphi|\lesssim35^{\circ}$ quoted in the main text is deliberately looser than all of these estimates.

Two further observations reinforce the conservative character of this bound. First, finite incident polarization and flipper efficiency give $r_{\mathrm{obs}}=\mathcal{P}_{\mathrm{eff}}r$, with $\mathcal{P}_{\mathrm{eff}}\leq1$, so the physical asymmetry is at least as large as the observed value and a polarization correction could only tighten the phase constraint. Second, the same interference relation gives an upper bound on the fraction of magnetic intensity that does not participate in the interference. Defining
\begin{equation}
f_{\perp}\equiv\frac{|M_{\perp,\not P}|^{2}}{|M_H|^{2}+|M_{\perp,\not P}|^{2}},
\end{equation}
one obtains
\begin{equation}
f_{\perp}\leq1-r^{2},
\end{equation}
with equality attained when $|M_H|/|N|=|r|$. We do not evaluate this expression using the largest observed asymmetry because of the selection bias discussed above.

Finally, these measurements cannot separately determine $N(T)$ and $M(T)$. Writing $S=a^{+}+a^{-}$ and $D=a^{+}-a^{-}$ gives $N^{2}+M^{2}=S/2$ and $NM=D/(4\cos\varphi)$, so the two amplitudes can formally be obtained as the roots of a quadratic at each temperature. This construction contains $2n$ unknown amplitudes for $2n$ observables, however, leaving no degrees of freedom; the resulting amplitudes therefore follow the measurement noise rather than providing an independent decomposition. Imposing a relation such as $N=KM^{p}$ restores $n-2$ degrees of freedom and permits a genuine model test, but the data do not select a particular scaling form. In particular, a temperature-independent nuclear amplitude is disfavored relative to the best fit by only $\Delta\chi^{2}=4.7$ for one additional constraint, a difference that does not remain significant after the twofold uncertainty inflation. We therefore make no claim as to whether the nuclear modulation is independently structural or magnetically induced. Debye--Waller damping does not affect this conclusion: at $L=1.65$, the momentum transfer is only $Q=0.240$~\AA$^{-1}$, for which the Debye--Waller factor exceeds $0.999$ even for $B=2$~\AA$^{2}$.

\section{Field-reduced symmetry analysis}

\begin{table}[H]
\caption{Transformation properties of the relevant quantities under the little co-group $m$ of $\bm q$.}
\label{tab:little-group}
\begin{ruledtabular}
\begin{tabular}{lcc}
quantity & under $m_x$ & irrep \\
\hline
$u_c(\bm q)$, displacement $\parallel\bm c$ & even & $\Lambda_1$ \\
$P_c(\bm q)$, polarization $\parallel\bm c$ & even & $\Lambda_1$ \\
$M_a(\bm q)$, moment $\parallel\bm H$ & even & $\Lambda_1$ \\
$M_c(\bm q)$, moment $\parallel\bm c$ & odd & $\Lambda_2$ \\
$M_b(\bm q)$, in-plane moment $\perp\bm H$ & odd & $\Lambda_2$ \\
$P_a(\bm q)$, polarization $\parallel\bm H$ & odd & $\Lambda_2$ \\
\end{tabular}
\end{ruledtabular}
\end{table}

The $\kTh$ state is stabilized only under an applied field, so the relevant parent symmetry is the subgroup of the paramagnetic grey group $R\bar{3}m1'$ that leaves the field invariant. Because $\bm H$ is an axial, time-odd vector, a unitary spatial operation $R$ preserves the applied field when $\det(R)R\bm H=\bm H$. Evaluating the twelve operations of $D_{3d}$ for $\hat{\bm x}\parallel\bm H\parallel[100]$ and $\hat{\bm z}\parallel\bm c$ leaves
\begin{equation}
\{E,\ C_{2x},\ \bar{1},\ m_x\},
\end{equation}
which form the unitary point group $2/m$ with its unique axis parallel to $\bm H$; in a field-adapted setting, this is the index-three monoclinic subgroup $C2/m$ of $R\bar{3}m$. None of the remaining spatial operations maps $\bm H$ exactly to $-\bm H$, so no additional symmetry is recovered by combining them with time reversal. The field-reduced symmetry is therefore the full point group $2/m$, rather than the mirror group alone. In particular, inversion survives because an axial vector is even under inversion, so the applied field does not by itself make the state polar. Of the four surviving operations, $E$ and $m_x=\bar{1}C_{2x}$ leave $\bm q=(0\,0\,q)$ invariant, whereas $C_{2x}$ and $\bar{1}$ exchange $\bm q$ and $-\bm q$. The little co-group of one arm of the propagation vector is therefore $m=\{E,m_x\}$, which has two one-dimensional representations: $\Lambda_1$, even under $m_x$, and $\Lambda_2$, odd under $m_x$. Axial vectors are transformed according to $\det(R)R\bm v$, giving the assignments listed in Table~\ref{tab:little-group}.

The longitudinal displacement, a possible longitudinal polarization, and the observed field-parallel magnetic component thus belong to the same representation, $\Lambda_1$, of the spatial little group. The observed modulation therefore lies in a symmetry channel that permits $P_c(\bm q)$, although symmetry alone does not establish that the structural mode is polar. Here, ``spatial'' refers specifically to transformations under crystallographic operations and does not include time reversal. The quantities $u_c$ and $P_c$ are time-even and polar, whereas $M_a$ is time-odd and axial; consequently, the bilinear $u_c^{*}M_a$ is time-odd and cannot appear by itself in a free energy invariant under simultaneous reversal of the magnetic variables and applied field. The required additional time-odd factor can be supplied by the uniform field-induced moment $M_0$, giving the coupling discussed in the main text.

To determine the allowed phase dependence, let $U\equiv u_c(\bm q)$, $M\equiv M_a(\bm q)$, and define $\delta\equiv\arg M-\arg U$. Under inversion, the conjugate arms are exchanged and the polar or axial character supplies the corresponding sign, so that $U\mapsto-U^{*}$ and $M\mapsto M^{*}$. It follows that $\mathrm{Im}(U^{*}M)$ is inversion-even, whereas $\mathrm{Re}(U^{*}M)$ is inversion-odd:
\begin{equation}
\mathrm{Im}(U^{*}M)=|U||M|\sin\delta\quad(\mathrm{even}),\qquad \mathrm{Re}(U^{*}M)=|U||M|\cos\delta\quad(\mathrm{odd}).
\end{equation}
The inversion-even combination gives the lowest-order magnetoelastic invariant
\begin{equation}
\mathcal{F}=i\lambda M_0\left(u_c^{*}M_a-u_cM_a^{*}\right)=-2\lambda M_0|u_c||M_a|\sin\delta,
\label{eq:flock}
\end{equation}
which is linear in both modulated amplitudes but requires $M_0\neq0$. The inversion-odd bilinear may instead enter when multiplied by another inversion-odd quantity. In particular,
\begin{equation}
\mathcal{F}_P=\gamma P_c(0)M_0\mathrm{Re}(U^{*}M)
\end{equation}
is symmetry-allowed and gives $P_c(0)\propto M_0|U||M|\cos\delta$ after minimization with respect to the uniform polarization. No second spatial representation is required because the polar--axial pairing itself makes $\mathrm{Re}(U^{*}M)$ inversion-odd. In a minimal single-mode model containing only these leading couplings, the magnetoelastic locking term and the uniform-polar response depend on complementary quadratures of the relative phase: the former is proportional to $\sin\delta$, whereas the latter is proportional to $\cos\delta$. This complementarity should not, however, be interpreted as a direct conclusion about the present sample.

There are two reasons why the measured phase cannot be used to predict $P_c(0)$. First, the measured nuclear--magnetic structure-factor phase is related to the order-parameter phase by
\begin{equation}
\varphi=\arg\!\left(N^{*}M_{\parallel H}\right)=\delta+\arg\!\left(S_N^{*}S_M\right)-\frac{\pi}{2},
\label{eq:phidelta}
\end{equation}
where $S_N=\sum_j b_jC_{N,j}e^{iGz_j}$ and $S_M=\sum_{j\in\mathrm{Fe}}p_mC_{M,j}e^{iGz_j}$ are the microscopic structural and magnetic basis sums for a single mode, with $u_j=C_{N,j}U$ and $M_j=C_{M,j}M$. These basis sums are unknown, and the separation between a basis phase and an order-parameter phase is gauge-dependent: the transformation $C_{N,j}\rightarrow e^{i\theta}C_{N,j}$, $U\rightarrow e^{-i\theta}U$ leaves the physical displacement unchanged while shifting the phase assigned to $U$. Thus, $\delta$ is meaningful only after a basis convention has been specified; in particular, the scalar-wave and inversion-adapted conventions used below differ by a quarter period. Second, the twelve-layer analysis in the following section shows that the structural order parameter has many independent directions. Several symmetry-allowed couplings with different coefficients and basis phases may therefore contribute, so a single scalar phase need not determine the uniform polarization.

At the superspace point-group level, five candidate symmetry classes remain under the assumptions of a single propagation vector, first-harmonic modulations, and no additional magnetic wavevector. We write a superspace operation as $\{g|\bm t;\tau\}$, where $\tau$ is an internal translation in units of the modulation period and $\tau=\tfrac{1}{2}$ reverses the sign of a first harmonic. Because the two experimentally established amplitudes transform as $\Lambda_1$, any candidate class that retains $m_x$ must contain it with $\tau=0$. Classes without $m_x$ remain possible if additional, experimentally unresolved symmetry-lowering amplitudes are present. The five resulting classes are summarized in Table~\ref{tab:superspace}.
\begin{table}[H]
\caption{Candidate magnetic superspace symmetry classes. The entries specify generator patterns at the superspace point-group level; formal Hermann--Mauguin superspace symbols would require transformation to the standard monoclinic setting and are not assigned here.}
\label{tab:superspace}
\begin{ruledtabular}
\begin{tabular}{llll}
class & generators & condition & uniform $P_c(0)$ \\
\hline
$G_{2/m}$ & $m_x(0),\,C_{2x}(\tau),\,\bar{1}(\tau)$ & $\Lambda_1$ only & forbidden \\
$G_m$ & $m_x(0)$ & $\Lambda_1$ only & allowed \\
$G_{\bar{1}}$ & $\bar{1}(\tau)$ & $\Lambda_1+\Lambda_2$ & forbidden \\
$G_2$ & $C_{2x}(\tau)$ & $\Lambda_1+\Lambda_2$ & forbidden; $P_a$ allowed \\
$G_1$ & translations only & generic $\Lambda_1+\Lambda_2$ & allowed \\
\end{tabular}
\end{ruledtabular}
\end{table}
In the generalized $2/m$ class, inversion combined with the appropriate internal translation forbids a uniform $P_c(0)$ while permitting a finite-wavevector $P_c(\bm q)$: the internal phase shift can compensate the transformation of a modulated polar quantity, whereas a uniform quantity has no internal phase. This class therefore provides a possible symmetry setting for a longitudinal polarization density wave and, as shown below, is compatible with the observed nuclear--magnetic interference without requiring an accidental structure-factor phase. The present data do not, however, distinguish it from the lower-symmetry $G_m$ class because that distinction depends on the unknown microscopic basis phases entering Eq.~\eqref{eq:phidelta}. The remaining three classes require an additional $\Lambda_2$ amplitude. The in-plane component $M_b$ is constrained by the bound on the noninterfering magnetic fraction derived above, whereas $M_c$ is projected out on the $(0\,0\,L)$ rod and therefore remains unconstrained by the present measurements.

\section{Twelve-layer eigenvector analysis}

The weak satellite around $\bm G=(0,\,0,\,0)$ can be analyzed using the refined crystal structure rather than a coarse-grained block model. We refer to the fitted constraint $\sum_j b_j u_{j,c}\simeq0$ as the near-extinction condition, emphasizing that it is an experimental upper bound rather than a systematic absence; the quantitative limit is derived in Sec.~\ref{sec:limit}. Folding the $4$~K refinement of Ref.~\onlinecite{Zhai2017} into one $c/3$ repeat, $0\leq z\leq1/6$, layers $j=2,\ldots,11$ form inversion-related pairs at $z$ and $\bar z=1/3-z$, whereas layers $1$ and $12$ lie on inversion-center planes. For each pair, we define coefficient-odd and coefficient-even displacement combinations, $O_j$ with $u(\bar z)=-u(z)$ and $E_j$ with $u(\bar z)=u(z)$, respectively. Because $u_c$ is a polar vector and transforms under inversion as $u_c(z)\mapsto-u_c(-z)$, their physical inversion characters are opposite to these coefficient labels: within this real, inversion-adapted symmetry slice, $O_j$ preserves inversion and is nonpolar, whereas $E_j$ breaks inversion and is capable of contributing to an inversion-breaking displacement modulation. A generic complex modulation admits additional displacement directions.



\begin{table}[t]
\caption{Symmetry-adapted basis of inversion-related layer pairs constructed from the $4$~K neutron refinement reported in Ref.~\onlinecite{Zhai2017}. The coefficients were evaluated using the unrounded refined coordinates and occupancies. A common factor of three from $R$ centering is omitted.}
\label{tab:pair}
\begin{ruledtabular}
\begin{tabular}{rlrrrrr}
$j$ & species & $z_j$ & $n_j$ & $w_j$ (fm) & $C^E_0,\ C^E_3$ & $A^O_3$ \\
\hline
1  & Fe    & $0$       & 1 & $9.450$  & $9.450,\ +9.450$   & --- \\
2  & O     & $0.02890$ & 3 & $17.409$ & $34.818,\ +29.778$ & $18.043$ \\
3  & Ba/Sr & $0.03553$ & 1 & $6.521$  & $13.041,\ +10.224$ & $8.096$ \\
4  & Fe    & $0.04277$ & 1 & $9.450$  & $18.900,\ +13.084$ & $13.639$ \\
5  & Fe    & $0.06500$ & 1 & $9.450$  & $18.900,\ +6.402$  & $17.783$ \\
6  & O     & $0.08587$ & 1 & $5.803$  & $11.606,\ -0.555$  & $11.593$ \\
7  & O     & $0.08440$ & 3 & $17.409$ & $34.818,\ -0.700$  & $34.811$ \\
8  & Fe/Mg & $0.10940$ & 3 & $24.854$ & $49.707,\ -23.453$ & $43.827$ \\
9  & O     & $0.13663$ & 1 & $5.803$  & $11.606,\ -9.795$  & $6.226$ \\
10 & O     & $0.13810$ & 3 & $17.409$ & $34.818,\ -29.891$ & $17.855$ \\
11 & Fe    & $0.15250$ & 1 & $9.450$  & $18.900,\ -18.230$ & $4.987$ \\
12 & Fe/Mg & $1/6$     & 1 & $8.272$  & $8.272,\ -8.272$   & --- \\
\end{tabular}
\end{ruledtabular}
\end{table}

The ten $O_j$ modes satisfy the $\bm G=(0,\,0,\,0)$ near-extinction condition identically because the contributions from each inversion-related pair cancel. The twelve $E_j$ amplitudes obey one real linear condition, $\sum_jC^E_{0,j}e_j=0$, leaving eleven independent combinations. Thus, even within this restricted real basis, the near-extinction-compatible displacement space contains $10+11=21$ independent directions. The finite nuclear amplitude inferred at $(0\,0\,3)$ excludes the subset for which the corresponding structure factor also vanishes, but it does not select a unique displacement eigenvector. We do not assign an exact dimension to this excluded subset because the number of independent conditions depends on the relative phase convention and on the superspace symmetry imposed on the $E_j$ and $O_j$ sectors.

The $O_8$ mode provides a particularly simple centrosymmetric solution consistent with the observed zone contrast. It displaces only the inversion-related Fe/Mg(8) planes at $z=0.1094$ and $0.2239$, both within $L$ blocks, and has a substantial $(0\,0\,3)$ structure factor, $|\widetilde F_3|=43.8$ in the reduced units of Table~\ref{tab:pair}. The existence of this intrablock solution demonstrates that the diffraction constraints neither require rigid $L$--$S$ antiphase motion nor determine a unique microscopic displacement pattern. Separately, the zone-contrast analysis in Sec.~\ref{sec:limit} excludes an acoustic-like rigid translation of the complete crystallographic basis and thereby establishes that the observed lattice response is an internal displacement mode.

The near-extinction condition also does not determine whether the mode carries a finite polarization, because neutron scattering lengths and Born effective charges define different linear combinations of the displacement eigenvector:
\begin{equation}
\sum_j b_j u_{j,c}\simeq0
\;\not\Rightarrow\;
Z^*_{\mathrm{mode}}
\equiv
\sum_j Z^*_{j,cc}u_{j,c}=0.
\end{equation}
In particular, the $O_j$ modes are explicit centrosymmetric solutions for which the mode effective charge vanishes by symmetry, showing that the present diffraction constraints do not require an inversion-breaking modulation. Refinement of satellites in additional Brillouin zones is needed to determine the displacement eigenvector and establish whether it preserves or breaks the relevant generalized inversion symmetry. Quantifying any associated finite-wavevector polarization additionally requires a linear-response calculation of the Born effective-charge tensors.

Finally, nuclear near-extinction does not imply magnetic extinction because the two structure factors involve different weights and atomic sublattices:
\begin{equation}
N(\bm G+\bm q)\propto iQ\sum_j b_j u_{j,c}e^{iGz_j},
\qquad
\bm M_{\perp}(\bm G+\bm q)\propto
\sum_{j\in\mathrm{Fe}}p_m f_j(Q)\bm\mu_{j,\perp}e^{iGz_j}.
\end{equation}
The nuclear sum includes all atomic layers, whereas the magnetic sum contains only the magnetic Fe sublattice. Consequently, the nuclear near-extinction condition places no corresponding extinction condition on the magnetic satellite at the same position.


%\bibliography{refs}



\end{document}
